# Supplementary material for: Invariance Through Latent Alignment
Source: arXiv:2112.08526 source file (2022-05-17)
Supplement: Supplementary file 1 [file generate_appendix.tex]

\documentclass{article} % For LaTeX2e
\usepackage{iclr2022_conference,times}

% Optional math commands from https://github.com/goodfeli/dlbook_notation.
\input{math_commands.tex}

\usepackage{xcolor}
\usepackage[colorlinks=true,citecolor=purple]{hyperref}
\usepackage{url}
\usepackage{algorithm}
\usepackage[noend]{algpseudocode}
\usepackage{enumitem}
\usepackage{graphicx}
\usepackage{caption}
\usepackage{subcaption}
\usepackage{xcolor}
\usepackage{xparse}
\usepackage{xspace}
\usepackage{xpatch}
\usepackage{tabularx}
\usepackage{booktabs}
\usepackage{makecell}
\usepackage{multirow}
\usepackage{multicol}
\usepackage{wrapfig}
\usepackage{tikz}
\usetikzlibrary{positioning,arrows.meta,fit,calc,backgrounds,decorations.pathmorphing}
\usepackage{tikzscale}

\usepackage{color}
\usepackage[textsize=scriptsize]{todonotes} % Add the 'disable' flag to hide comments
\setlength{\marginparsep}{0.1cm}
\setlength{\marginparwidth}{3.5cm}

\title{Invariance Through Inference}
% \title{Revisiting Neural Value Approximation with Fourier}

% Authors must not appear in the submitted version. They should be hidden
% as long as the \iclrfinalcopy macro remains commented out below.
% Non-anonymous submissions will be rejected without review.

\author{Antiquus S.~Hippocampus, Natalia Cerebro \& Amelie P. Amygdale \thanks{ Use footnote for providing further information
about author (webpage, alternative address)---\emph{not} for acknowledging
funding agencies.  Funding acknowledgements go at the end of the paper.} \\
\texttt{\{hippo,brain,jen\}@cs.cranberry-lemon.edu} \\
}

% The \author macro works with any number of authors. There are two commands
% used to separate the names and addresses of multiple authors: \And and \AND.
%
% Using \And between authors leaves it to \LaTeX{} to determine where to break
% the lines. Using \AND forces a linebreak at that point. So, if \LaTeX{}
% puts 3 of 4 authors names on the first line, and the last on the second
% line, try using \AND instead of \And before the third author name.

\definecolor{mydarkblue}{rgb}{0,0.08,0.45}
\definecolor{es-blue}{rgb}{0,0.4,0.8}

\usepackage{siunitx}
\sisetup{separate-uncertainty}
%\iclrfinalcopy % Uncomment for camera-ready version, but NOT for submission.
\begin{document}

\input{sections/appendix}

% \clearpage

% \bibliography{references.bib}
% \bibliographystyle{iclr2022_conference}

%\appendix
%\section{Appendix}
%You may include other additional sections here.

\end{document}
