# Supplementary material for: Invariance Through Latent Alignment
Source: arXiv:2112.08526 source file (2022-05-17)
Supplement: Supplementary file 2 [file supplementary.tex]

\documentclass[main.tex]{subfiles}

\begin{document}

% paper title
\title{Invariance Through Inference\\%
{\Large Supplementary Material}}

% You will get a Paper-ID when submitting a pdf file to the conference system
\author{Author Names Omitted for Anonymous Review. Paper-ID 175}

\onecolumn

\maketitle
\input{sections/appendix}

\bibliography{references}
\bibliographystyle{IEEEtranN}

\end{document}
